# Supplementary material for: On the Nonlinear Eshelby Inclusion Problem and its Isomorphic Growth Limit
Source: arXiv:2411.04948 source file (2024-11-07)
Supplement: Supplementary file 2 [file AppendixCdel.tex]

  % redefine the command that creates the equation no.
  \setcounter{equation}{0}  % reset counter   \section*{Appendix A: TEST}  % use *-form to suppress numbering
  \section*{Appendix C: Derivation of the Equations for an Elliptic Cylinder in the Isomorphic Limit}  % use *-form to suppress numbering
