# Supplementary material for: On the Nonlinear Eshelby Inclusion Problem and its Isomorphic Growth Limit
Source: arXiv:2411.04948 source file (2024-11-07)
Supplement: Supplementary file 3 [file AppendixD.tex]

  % redefine the command that creates the equation no.
  \setcounter{equation}{0}  % reset counter   \section*{Appendix A: TEST}  % use *-form to suppress numbering
  
  % redefine the command that creates the equation no.
  \setcounter{figure}{0}  % reset counter   \section*{Appendix A: TEST}  % use *-form to suppress numbering
  \section*{Appendix D: Details of Finite Element Simulations}  % use *-form to suppress numbering

  The axisymmetric simulations were run using a quarter elliptical mesh the same aspect ratio as the inclusion with an outer radius 1000 times $A_1$. The mesh was partitioned into the matrix and inclusion, and a residual was enforced which caused the inclusion to grow isotropically, by enforcing a $J^*_I\neq1$. \textcolor{red}{CHECK THIS WITH CHOCKA. CITE PAPERS?}
